# Supplementary material for: Knowledge Regularized Negative Feature Tuning of Vision-Language Models for Out-of-Distribution Detection
Source: arXiv:2507.19847 source file (2025-07-29)
Supplement: Supplementary file 1 [file X_suppl.tex]

\setcounter{page}{1}

The following contents are provided in this supplementary material:
\begin{itemize}
	\item Different strategies that introduce negative training samples (\cf Sec. 3.2).
        \item More detailed results of OOD detection for ID of ImageNet-1k. (\cf Tab. 1).
        \item More detailed results of OOD detection on unseen classes (\cf Tab. 2).
        \item More detailed results of OOD detection on unseen styles (\cf Tab. 3).
        \item Knowledge Regularization Implementations. (\cf Sec. 4.3)
        \item More analyses and discussions. (\cf Sec. 4.3)
\end{itemize}

\section{Different strategies that introduce negative training samples (\cf Sec. 4.3).} \label{sec:different_negative_strategy}
Besides generating negative training samples with cropping and selection as detailed in the main paper, we also validate that our method is also compatible with other strategies that introduce negative training samples.
Specifically, following \cite{miyai2024locoop}, we generate local features set $X_k^{local} = \{ \vx_{k,1}^{local}, ..., \vx_{k,P}^{local}\}$ from $\vx_k$, where $P$ is the number of local features. 
Given these image local features, we calculate their cosine similarities to the text feature of the corresponding label, \eg, `a photo of a $<y_k>$.'. We define local features with the highest and lowest similarity as $X_k^{p} = \{ \vx_{k,1}^{p}, \ldots, \vx_{k,Q}^{p}\}$ and $X_k^{n} = \{ \vx_{k,1}^{n}, \ldots, \vx_{k,Q}^{n}\}$, where Q is the hyperparameter determining the number of selected local features. Finally, we collect the training data as $\mathcal{D}_{p} = \{(\vx_{1,1}^{p}, y_1^{p}), (\vx_{1,2}^{p}, y_1^{p}), \ldots, (\vx_{K,Q}^{p}, y_K)\}$ and $\mathcal{D}_{n} = \{(\vx_{1,1}^{n}, \vx_{1,2}^{n}, \ldots, \vx_{K,Q}^{n})\}$.
As shown in Tab. \ref{tab:neg_samples}, our method can consistently outperform the pre-trained VLMs with different strategies that introduce negative training samples.

% We use CLIP score to measure cosine similarity to the corresponding text feature and select the top-Q local features and bottom-Q features as $X_k^{p} = \{ \vx_{k,1}^{p}, \ldots, \vx_{k,Q}^{p}\}$ and $X_k^{n} = \{ \vx_{k,1}^{n}, \ldots, \vx_{k,Q}^{n}\}$, the local training data can be denoted as $\mathcal{D}_{p} = \{(\vx_{1,1}^{p}, y_1^{p}), (\vx_{1,2}^{p}, y_1^{p}), \ldots, (\vx_{K,Q}^{p}, y_K)\}$ and $\mathcal{D}_{n} = \{(\vx_{1,1}^{n}, \vx_{1,2}^{n}, \ldots, \vx_{K,Q}^{n})\}$. 

% As shown in Tab. \ref{tab:neg_samples}, our method can also achieves impressive ood detection performance with other negative samples strategies. 

\begin{table}[H]
    \centering
        \centering
        \begin{tabular}{l|ccc}
        \toprule
        Method & \multicolumn{3}{c}{FPR95 $\downarrow$} \\
        & Base & New & H-MEAN \\
        \midrule
        NegLabel & 25.40 & 12.15 & 16.45 \\
        \hline
        KR-NFT (Crops) & 22.79 & 11.41 & 15.21 \\
        KR-NFT (Local Features) & 24.82 & 10.02 & 14.28 \\
        \bottomrule
        \end{tabular}
        \caption{Results with different strategies that generate negative samples. KR-NFT (Crops) is the strategy illustrated in the main text which generates and selects random crops as training data. KR-NFT (Local Features)  refers to the strategy of selecting local features as negative training samples, which is detailed in Sec. \ref{sec:different_negative_strategy}.}
        \label{tab:neg_samples}
        \vspace{-0.4cm}
    \hfill
\end{table}

\section{More detailed results of OOD detection for ID of ImageNet-1k. (\cf Tab. 1).}
The detailed results of OOD detection for ID of ImageNet-1k are presented in Tab. \ref{tab:imagenet_ood}.

\section{More detailed results of OOD detection on unseen classes (\cf Tab. 2).}
The detailed results of OOD detection for ID of CIFAR10, CIFAR100 and Fine-grained datasets are presented in Tab. \ref{tab:cifar_ood}, and Tab. \ref{tab:fine_grained_ood} respectively. Our KR-NFT outperforms other methods on the three datasets with unseen classes, illustrating its strong generalization capabilities for unseen class OOD detection.

\section{More detailed results of OOD detection on unseen styles (\cf Tab. 3).}
The detailed results of OOD detection for ID of unseen styles are presented in Tab. \ref{tab:cross_domain_ood}. Our KR-NFT outperforms other methods on the four unseen styles datasets, validating its strong generalization capabilities for unseen styles OOD detection.

\section{Knowledge Regularization Implementations}
We also explore different implementations of the knowledge regularization objectives, besides the one used in Eq. (7) of the main paper.  
Specifically, we apply the knowledge regularization objective on the logits (\eg, $\mC'\vv$) with the following equation:
% The knowledge preservation objective for the logits (\eg, $\mC'\vv$) 
% is shown in Eq. \ref{eq:kp_logits}: 
\begin{equation}\label{eq:kp_logits}
\mathcal{L}_{\text {kr(logits)}} = \frac{1}{N+M} \sum_{i=1}^{N+M} \left(\vc_i \vv - \vc_i' \vv \right)^2,
\end{equation}
where $\vc_i' \vv \in \mathcal{R}$ denotes the cosine similarity between the image feature $\vv$ and text feature $\vc_i$.

We also apply the knowledge regularization objective on the probabilities (\eg, Softmax($\mC'\vv$)) with the following equation:
% The knowledge preservation objective for the probabilities (\eg, Softmax($\mC'\vv$)) is shown in Eq. \ref{eq:kp_prob} :
\begin{equation}\label{eq:kp_prob}
\mathcal{L}_{\text {kr(prob)}} =  -\sum_{i=1}^{N+M} \frac{e^{\cos(\vv, \vc_i)}}{\sum_{j=1}^{N+M} {e^{\cos(\vv, \vc_j)}}}  \log(\frac{e^{\cos(\vv, \vc_i')}}{\sum_{j=1}^{N+M} {e^{\cos(\vv, \vc_j')}}} ),
\end{equation}
where the temperature scaling parameter is omitted for simplicity.

\section{More Analyses and Discussions.}

\noindent \textbf{Different backbone architectures.}
Results of OOD detection using different backbone architectures are shown in the Tab. \ref{tab:backbones}. The results indicate that our KR-NFT can perform well on different backbone architectures, and stronger backbones lead to better performance.
\begin{table}[H]
    \centering
        \centering
        \begin{tabular}{l|lccc}
        \toprule
        Backbone & Method & \multicolumn{3}{c}{FPR95 $\downarrow$} \\
        & & Base & New & H-MEAN \\
        \midrule
         \multirow{2}{*}{ResNet50} & NegLabel & 28.70 & 35.05 & 31.56 \\
          & KR-NFT & 28.06 & 34.72 & 31.05 \\
        \midrule
         \multirow{2}{*}{VITB/16} & NegLabel & 25.40 & 12.15 & 16.45 \\
          & KR-NFT & 22.79 & 11.41 & 15.21 \\
         \multirow{2}{*}{VITL/14} & NegLabel & 24.81 & 11.96 & 18.39 \\
          & KR-NFT & 21.04 & 6.86 & 10.42 \\ 
        \bottomrule
        \end{tabular}
        \caption{Results with different backbone architectures. }
        \label{tab:backbones}
        \vspace{-0.5cm}
    \hfill
\end{table}

\noindent \textbf{Different training shots.}
Results of OOD detection using different training shots are shown in Tab. \ref{tab:shots}. The results indicate that better performance can be achieved with more training samples.
\begin{table}[ht]
    \centering
        \centering
        \begin{tabular}{l|ccc}
        \toprule
        Training shots & \multicolumn{3}{c}{FPR95 $\downarrow$} \\
        & Base & New & H-MEAN \\
        \midrule
         One-shot & 23.40 & 12.66 & 16.45 \\
         Four-shot & 22.79 & 11.41 & 15.21 \\
        \bottomrule
        \end{tabular}
        \caption{Results with different training shots. }
        \label{tab:shots}
        \vspace{-0.8cm}
    \hfill
\end{table}

\noindent \textbf{Different training datasets.} Results of OOD detection using different training datasets are shown in Tab. \ref{tab:training_dataset}. 
Using a larger training dataset, such as ImageNet, can lead to better generalization performance. Therefore, we recommend using the ImageNet dataset as the training data for enhanced generalization capabilities.

%Though the model trained on CIFAR10 achieves better results on CIFAR100 OOD detection, it performs worse than NegLabel in OOD detection on unseen styles. The model trained on ImageNet performs well in OOD detection for unseen classes and styles. This indicates that models need to leverage large-scale datasets for training to improve their comprehensive OOD detection capabilities.  
\begin{table}[H]
\small
    \centering
        \centering
        \begin{tabular}{l|cc}
        \toprule
        Training dataset & \multicolumn{2}{c}{FPR95 $\downarrow$} \\
         & Fine-grained & Unseen styles \\
        \midrule
         NegLabel  & 41.28 & 30.26 \\
        \midrule
         CIFAR10  & 40.95 & 45.31 \\
         ImageNet & 40.33 & 28.13 \\
        \bottomrule
        \end{tabular}
        \caption{The OOD detection results on unseen classes and styles, where models are trained with different training datasets.}
        \label{tab:training_dataset}
    \hfill
\end{table}

\vspace{-0.6cm}
\noindent \textbf{Different feature tuning instantiations}
We analyzed the feature tuning function with varying complexities. The simplest transformation adds a learnable constant value $\beta\in\mathcal{R}$ to the text vector, resulting in `$L_2 (\vc_i + \beta)$'. We also tried adding an element-wise vector $\bm{\beta} \in \mathcal{R}^D$ to the text vector, similar to TaskRes \cite{yu2023task}, leading to `$L_2 (\vc_i + \bm{\beta})$'. Our proposed method involves element-wise scaling and shifting of the text feature, expressed as `$L_2 (\bm{\alpha} \vc_i + \bm{\beta})$'. Additionally, we experimented with a more complex approach using a two-layer MLP for feature transformation, \ie, `$L_2 (MLP(\vc_i ))$'.
We carefully initialize learnable parameters to ensure that at the beginning of training $T(\vc_i) = \vc_i$, avoiding disturbing pre-trained knowledge.
As shown in Tab. \ref{tab:functions}, our approach yielded the best results. Simpler transformations like `$L_2 (\vc_i + \beta)$' lacked sufficient capability, as evidenced by the limited improvement in Base classes. Conversely, more complex transformations such as `$L_2 (MLP(\vc_i ))$' tended to overfit, as validated by the reduced generalization performance on the New classes.

\begin{table}[H]
    \centering
        \centering
        \begin{tabular}{l|ccc}
        \toprule
        {\multirow{2}{*}{$T(\vc_i)$=}} & \multicolumn{3}{c}{FPR95 $\downarrow$} \\
        & Base & New & H-MEAN \\
        \midrule
        Prompt Learning & 24.21 & 27.33 & 25.68 \\
        \midrule
        $L_2 (\vc_i + \beta)$ & 24.87 & 26.42 & 25.64 \\
        $L_2 (\vc_i + \bm{\beta})$ & 25.01 & 26.35 & 25.66 \\
        $L_2 (\bm{\alpha} \vc_i + \bm{\beta})$ (Ours) & 25.02 & 26.08  & 25.54 \\
        $L_2 (MLP(\vc_i ))$ & 24.12 & 31.61 & 27.39 \\ %% your MLP transformation
        \bottomrule
        \end{tabular}
        \caption{Results with different implementations of the feature tuning, where the ImageNet and CIFAR10 are adopted as the Base and New settings, respectively. }
        \label{tab:functions}
    \hfill
\end{table}

\begin{table*}[ht] 
\small
\centering
% \vspace{-0.2cm}
\begin{tabular}{lcccccccc|cc}
\toprule
\multicolumn{11}{c}{OOD datasets}  \\
\multicolumn{1}{c}{{Methods}} & \multicolumn{2}{c}{INaturalist} & \multicolumn{2}{c}{SUN} & \multicolumn{2}{c}{Places} & \multicolumn{2}{c}{Textures} & \multicolumn{2}{c}{Average} \\ \cline{2-3} \cline{4-5} \cline{6-7} \cline{8-9} \cline{10-11}
 & \fontsize{8}{12}\selectfont AUROC$\uparrow$ & \fontsize{8}{12}\selectfont FPR95$\downarrow$& \fontsize{8}{12}\selectfont AUROC$\uparrow$ & \fontsize{8}{12}\selectfont FPR95$\downarrow$& \fontsize{8}{12}\selectfont AUROC$\uparrow$ & \fontsize{8}{12}\selectfont FPR95$\downarrow$& \fontsize{8}{12}\selectfont AUROC$\uparrow$ & \fontsize{8}{12}\selectfont FPR95$\downarrow$ & \fontsize{8}{12}\selectfont AUROC$\uparrow$ & \fontsize{8}{12}\selectfont FPR95$\downarrow$  \\
 \midrule
  \multicolumn{11}{c}{\textbf{Zero Shot (No Training Required)}} \\
Mahalanobis \cite{lee2018simple} & 55.89 & 99.33 & 59.94 & 99.41 & 65.96 & 98.54 & 64.23 & 98.46 & 61.50 & 98.94 \\
Energy \cite{liu2020energy} & 85.09 & 81.08 & 84.24 & 79.02 & 83.38 & 75.08 & 65.56 & 93.65 & 79.57 & 82.21 \\
MCM \cite{ming2022delving} & 94.59 & 32.20 & 92.25 & 38.80 & 90.31 & 46.20 & 86.12 & 58.50 & 90.82 & 43.93 \\
EOE \cite{cao2024envisioning} & 97.52 & 12.29 & 95.73 & 20.40 &  92.95 & 30.16 & 85.64 & 57.63 & 92.96 & 30.09 \\
NegLabel \cite{jiang2024negative} & 99.49 & 1.91 & 95.49 & 20.53 & 91.64 & 35.59 & 90.22 & 43.56 & 94.21 & 25.40 \\
\midrule
  \multicolumn{11}{c}{\textbf{Training-required (or with Fine-tuning)}} \\ 
MSP \cite{hendrycks2016baseline} & 87.44 & 58.36 & 79.73 & 73.72 & 79.67 & 74.41 & 79.69 & 71.93 & 81.63 & 69.61   \\
ODIN \cite{liang2017enhancing} & 94.65 & 30.22 & 87.17 & 54.04 & 85.54 & 55.06 & 87.85 & 51.67 & 88.80 & 47.75   \\
Energy \cite{liu2020energy} & 95.33 & 26.12 & 92.66 & 35.97 & 91.41 & 39.87 & 86.76 & 57.61 & 91.54 & 39.89 \\
GradNorm \cite{huang2021importance} & 72.56 & 81.50 & 72.86 & 82.00 & 73.70 & 80.41 & 70.26 & 79.36 & 72.35 & 80.82 \\
ViM \cite{wang2022vim} & 93.16 & 32.19 & 87.19 & 54.01 & 83.75 & 60.67 & 87.18 & 53.94 & 87.82 & 50.20 \\
KNN \cite{sun2022dice} & 94.52 & 29.17 & 92.67 & 35.62 & 91.02 & 39.61 & 85.67 & 64.35 & 90.97 & 42.19 \\
VOS \cite{du2022unknown} & 94.62 & 28.99 & 92.57 & 36.88 & 91.23 & 38.39 & 86.33 & 61.02 & 91.19 & 41.32 \\
NPOS \cite{tao2023non} & 96.19 & 16.58 & 90.44 & 43.77 & 89.44 & 45.27 & 88.80 & 46.12 & 91.22 & 37.93\\  
ZOC \cite{esmaeilpour2022zero} & 86.09 & 87.30 & 81.20 & 81.51 & 83.39 & 73.06 & 76.46 & 98.90 & 81.79 & 85.19 \\
CLIPN \cite{wang2023clipn} & 95.27 & 23.94 & 93.93 & 26.17 & 92.28 & 33.45 & 90.93 & 40.83 & 93.10 & 31.10 \\
LoCoOp \cite{miyai2024locoop} & 93.93 & 29.45 & 90.32 & 41.13 & 90.54 & 44.15 & 93.24 & 33.06 & 92.01 & 36.95 \\
ID-Like \cite{bai2024id} & 98.19 & 8.98 & 91.64 & 42.03 & 90.57 & 44.00 & \textbf{94.32} & \textbf{25.27} & 93.68 & 30.07 \\
NegPrompt \cite{li2024learning} & 90.49 & 37.79 & 92.25 & 32.11 & 91.16 & 35.52 & 88.38 & 43.93 & 90.57 & 37.34 \\
SCT \cite{yu2024self} & 95.86 & 13.94 & 95.33 & 20.55 & 92.24 & 29.86 & 89.06 & 41.51 & 93.37 & 26.47 \\
LAPT \cite{zhang2024lapt} & 99.63 & \textbf{1.16} & 96.01 & 19.12 & 92.01 & 33.01 & 91.06 & 40.32 & 94.68 & 23.40 \\
\rowcolor{lightpink} 
\textbf{KR-NFT (Ours)} & 99.62 & \textbf{0.82} & 96.15 & 17.83 & 92.64 & 36.12 & 91.96 & 36.38 & 95.09 & 22.79 \\
\textbf{KR-NFT} ($\lambda_2$=0) & \textbf{99.67} & 1.33 & \textbf{96.28} & \textbf{17.46} & \textbf{93.68} & \textbf{28.17} & 93.26 & 29.34 & \textbf{95.82} & \textbf{19.08} \\
\bottomrule
\end{tabular}
\caption{OOD detection results for ID of ImageNet-1k using a VITB/16 encoder. }
\vspace{-0.2cm}
\label{tab:imagenet_ood}
\end{table*}

\begin{table*}[ht]
\centering
% \vspace{-0.2cm}
\begin{tabular}{lllccccccc|ccc}
\toprule
\multicolumn{12}{c}{OOD datasets}  \\
\multicolumn{1}{c}{\multirow{2}{*}{ID Dataset}} & \multicolumn{1}{c}{\multirow{2}{*}{Methods}} & \multicolumn{2}{c}{MNIST} & \multicolumn{2}{c}{SVHN} & \multicolumn{2}{c}{Places} & \multicolumn{2}{c}{Textures} & \multicolumn{2}{c}{Average} \\ \cline{3-4} \cline{5-6} \cline{6-7} \cline{8-9} \cline{10-12}
 & & \tiny AUROC$\uparrow$ & \tiny FPR95$\downarrow$ & \tiny AUROC$\uparrow$ & \tiny FPR95$\downarrow$ & \tiny AUROC$\uparrow$ & \tiny FPR95$\downarrow$ & \tiny AUROC$\uparrow$ & \tiny FPR95$\downarrow$ & \tiny AUROC$\uparrow$ 
 & \tiny FPR95$\downarrow$ \\
 \midrule
{\multirow{7}{*}{CIFAR10}} & MCM \cite{ming2022delving} & 99.36 & 1.97 & 99.36 & 2.68 & 96.74 & 39.38 & 92.25 & 13.11 & 96.93 & 14.28 \\  
& NegLabel \cite{jiang2024negative} & 95.52 & 7.85 & 96.32 & 9.06 & 97.46 & 10.25 & 95.77 & 21.44 & 96.27 & 12.15 \\ 
& LoCoOp \cite{miyai2024locoop} & 98.63 & 5.72 & 98.83 & 3.69 & 91.45 & 36.02 & 85.55 & 59.99 & 93.61 & 26.36 \\
& ID-Like \cite{bai2024id} & 90.14 & 18.73 & 90.42 & 18.75 & 32.09 & 99.86 & 63.42 & 82.64 & 69.02 & 54.99 \\
& NegPrompt \cite{li2024learning} & 97.98 & 7.00 & 98.13 & 6.42 & 94.25 & 28.70 & 80.81 & 74.71 & 92.79 & 29.21 \\
& SCT \cite{yu2024self} & 98.58 & 0.49 & 97.71 & 5.45 & 88.85 & 44.96 & 95.53 & 22.23 & 95.17 & 18.28 \\
& LAPT \cite{zhang2024lapt} & 96.08 & 6.99 & 94.30 & 12.69 & 98.61 & 5.90 & 93.05 & 43.44 & 95.51 & 17.26 \\
& \textbf{KR-NFT} & 96.23 & 6.64 & 97.54 & 6.43 & 97.70 & 10.58 & 95.79 & 22.00 & \textbf{96.82} & \textbf{11.41} \\
 \midrule
{\multirow{7}{*}{CIFAR100}}
& MCM \cite{ming2022delving} & 92.09 & 21.28 & 88.64 & 29.54 & 63.57 & 85.60 & 74.59 & 77.44 & 79.72 & 53.46 \\  
& NegLabel \cite{jiang2024negative} & 83.15 & 29.32 & 77.74 & 43.78 & 79.64 & 74.12 & 82.13 & 68.98 & 80.66 & 54.05 \\ 
& LoCoOp \cite{miyai2024locoop} & 94.24 & 19.53 & 93.19 & 29.71 & 60.42 & 85.67 & 46.28 & 93.21 & 73.53 & 57.03 \\
& ID-Like \cite{bai2024id} & 85.44 & 29.65 & 85.51 & 32.78 & 8.84 & 99.93 & 26.07 & 99.33 & 51.46 & 65.44 \\
& NegPrompt \cite{li2024learning} & 91.54 & 23.78 & 85.61 & 44.40 & 75.41 & 88.50 & 54.71 & 97.07 & 76.82 & 63.44 \\
& SCT \cite{yu2024self} & 96.23 & 25.26 & 95.24 & 31.00 & 50.28 & 99.82 & 68.46 & 95.88 & 77.55 & 62.99 \\
& LAPT \cite{zhang2024lapt} & 81.35 & 33.37 & 76.77 & 52.13 & 88.17 & 59.30 & 69.47 & 83.65 & 78.94 & 57.11 \\
& \textbf{KR-NFT} & 90.00 & 19.33 & 86.64 & 30.98 & 75.58 & 79.28 & 70.39 & 83.39 & 80.65 & 53.24 \\
\bottomrule
\end{tabular}
\caption{Transfer to CIFAR10/CIFAR100 OOD detection results with ID data of ImageNet-1k and four OOD datasets by using the VITB/16 CLIP encoder.} \label{tab:cifar_ood}
% \vspace{-0.2cm}
\end{table*}

\begin{table*}[ht] \scriptsize
\centering
\begin{tabular}{lccccccccc|cc}
\toprule
{\multirow{3}{*}{Method}} & ID & \multicolumn{2}{c}{CUB-100} & \multicolumn{2}{c}{Stanford-Cars-98} & \multicolumn{2}{c}{Food-50} & \multicolumn{2}{c}{Oxford-Pet-18} & \multicolumn{2}{c}{Average} \\
& OOD & \multicolumn{2}{c}{CUB-100} & \multicolumn{2}{c}{Stanford-Cars-98}
& \multicolumn{2}{c}{Food-51} & \multicolumn{2}{c}{Oxford-Pet-19} & \\
\midrule
&  & AUROC $\uparrow$ & FPR95 $\downarrow$ & AUROC $\uparrow$ & FPR95 $\downarrow$ & AUROC $\uparrow$ & FPR95 $\downarrow$ & AUROC $\uparrow$ & FPR95 $\downarrow$ & AUROC $\uparrow$ & FPR95 $\downarrow$ \\
\midrule
MCM \cite{ming2022delving} &  &67.51  &83.58  &68.71 &83.99  &91.75  &43.38  &84.88  &63.92  &78.21  &68.72  \\
NegLabel \cite{jiang2024negative} &  &89.58  &42.00  &92.14 &40.15  &90.30 &40.89  &87.94 &42.09  &89.99 &41.28  \\
LoCoOp \cite{miyai2024locoop} &  &50.92 &91.17  &63.76  &82.68  &76.17  &71.11  &47.05  &92.14  &59.48  &84.28 \\
ID-Like \cite{bai2024id} &  &81.33  &63.50  &81.99  &57.40  &84.78  &57.60  &80.70  &65.88  &82.20  &61.10   \\
NegPrompt \cite{li2024learning} &  & 76.21 & 71.17 & 72.25 & 74.73 & 79.23 & 69.97 & 83.67 & 57.40 & 78.83 & 68.32 \\
SCT \cite{yu2024self} &  & 83.45 & 66.59 & 77.60 & 70.58 & 88.71 & 54.55 & 82.69 & 69.05 & 83.11 & 65.09 \\
LAPT \cite{zhang2024lapt} &  & 90.63 & 38.13 & 91.16 & 44.98 & 91.02 & 39.70 & 90.41 & 38.16 & 90.85 & 40.24 \\
KR-NFT  &  & 88.64 & 44.50 & 92.32 & 38.28 & 89.46 & 42.46 & 88.49 & 40.01 & 89.99 & 40.33  \\
\bottomrule
\end{tabular}
\caption{Transfer to Fine-grained ood detection results with ID data of ImageNet-1k and four OOD datasets by using the VITB/16 CLIP encoder.}
\label{tab:fine_grained_ood}
\end{table*}}

\begin{table*}[ht]
\centering
% \vspace{-0.2cm}
\begin{tabular}{llcccccccc|ccc}
\toprule
\multicolumn{12}{c}{OOD datasets}  \\
\multicolumn{1}{c}{\multirow{2}{*}{ID Dataset}} & \multicolumn{1}{c}{\multirow{2}{*}{Methods}} & \multicolumn{2}{c}{INaturalist} & \multicolumn{2}{c}{SUN} & \multicolumn{2}{c}{Places} & \multicolumn{2}{c}{Textures} & \multicolumn{2}{c}{Average} \\ \cline{3-4} \cline{5-6} \cline{6-7} \cline{8-9} \cline{10-12}
 & & \tiny AUROC$\uparrow$ & \tiny FPR95$\downarrow$& \tiny AUROC$\uparrow$ & \tiny FPR95$\downarrow$& \tiny AUROC$\uparrow$ & \tiny FPR95$\downarrow$& \tiny AUROC$\uparrow$ & \tiny FPR95$\downarrow$ & \tiny AUROC$\uparrow$ & \tiny FPR95$\downarrow$   \\
 \midrule
{\multirow{5}{*}{ImageNet-S}} & MCM  & 87.74 & 63.06 & 85.35 & 67.24 & 81.19 & 70.64 & 74.77 & 79.59 & 82.26 & 70.13 \\  
& NegLabel \cite{jiang2024negative} & 99.34 & 2.24 & 94.93 & 22.73 & 90.78 & 38.62 & 89.29 & 46.10 & 93.59 & 27.42 \\ 
& LoCoOp \cite{miyai2024locoop} & 59.61 & 71.52 & 68.91 & 73.18 & 66.51 & 81.22 & 78.23 & 67.50 & 68.32 & 73.35 \\
& ID-Like \cite{bai2024id} & 92.25 & 44.44 & 80.02 & 75.72 & 82.76 & 70.16 & 89.47 & 42.45 & 86.13 & 58.19 \\
& NegPrompt \cite{li2024learning} & 75.97 & 63.98 & 73.99 & 70.06 & 79.45 & 64.07 & 80.88 & 62.62 & 77.57 & 65.18 \\
& SCT \cite{yu2024self} & 89.80 & 42.28 & 88.96 & 46.59 & 83.90 & 55.46 & 77.67 & 68.88 & 85.11 & 53.30 \\
& LAPT \cite{zhang2024lapt} & 98.20 & 7.03 & 85.03 & 55.71 & 79.89 & 70.40 & 76.06 & 74.36 & 84.80 & 51.87 \\
& \textbf{KR-NFT} & 99.32 & 2.38 & 94.68 & 24.39 & 91.50 & 33.67 & 90.91 & 38.81 & 94.10 & 24.81 \\
 \midrule
{\multirow{5}{*}{ImageNet-A}}
& MCM \cite{ming2022delving} & 79.50 & 76.85 & 76.19 & 79.78 & 70.95 & 80.51 & 61.98 & 86.37 & 72.16 & 80.88 \\  
& NegLabel \cite{jiang2024negative} & 98.80 & 4.09 & 89.83 & 44.38 & 82.88 & 60.10 & 80.25 & 64.34 & 87.94 & 43.23 \\ 
& LoCoOp \cite{miyai2024locoop} & 67.08 & 80.37 & 76.31 & 69.00 & 72.70 & 84.50 & 74.54 & 76.70 & 72.66 & 77.64 \\
& ID-Like \cite{bai2024id} & 78.55 & 79.50 & 57.64 & 93.45 & 61.77 & 90.78 & 76.12 & 67.64 & 68.52 & 82.84 \\
& NegPrompt \cite{li2024learning} & 64.38 & 77.52 & 63.56 & 83.61 & 71.88 & 77.10 & 79.45 & 68.04 & 69.82 & 76.57 \\
& SCT \cite{yu2024self} & 86.38 & 53.11 & 85.08 & 57.78 & 78.96 & 65.26 & 70.77 & 76.38 & 80.30 & 63.13 \\
& LAPT \cite{zhang2024lapt} & 98.84 & 4.25 & 87.95 & 52.13 & 82.72 & 74.17 & 79.20 & 75.33 & 87.18 & 51.47 \\
& \textbf{KR-NFT} & 98.72 & 4.31 & 89.63 & 43.62 & 84.77 & 49.94 & 83.42 & 55.98 & 89.13 & 38.46 \\
 \midrule
{\multirow{5}{*}{ImageNet-R}} & MCM \cite{ming2022delving} & 83.22 & 71.51 & 80.31 & 74.98 & 75.53 & 76.67 & 67.66 & 83.72 & 76.68 & 76.72 \\  
& NegLabel \cite{jiang2024negative} & 99.58 & 1.60 & 96.03 & 15.77 & 91.97 & 29.48 & 90.60 & 35.67 & 94.54 & 20.63 \\ 
& LoCoOp \cite{miyai2024locoop} & 23.79 & 96.40 & 51.12 & 89.01 & 52.74 & 92.25 & 73.78 & 78.88 & 50.36 & 89.14 \\
& ID-Like \cite{bai2024id} & 90.64 & 48.39 & 75.54 & 78.22 & 78.82 & 72.90 & 87.33 & 44.86 & 83.08 & 61.09\\
& NegPrompt \cite{li2024learning} & 78.71 & 51.76 & 77.85 & 58.50 & 80.45 & 62.78 & 85.80 & 51.01 & 80.70 & 56.01 \\
& SCT \cite{yu2024self} & 90.33 & 37.64 & 89.34 & 41.57 & 83.99 & 50.72 & 77.28 & 65.31 & 85.23 & 48.81 \\
& LAPT \cite{zhang2024lapt} & 98.97 & 3.99 & 88.42 & 49.18 & 83.52 & 68.02 & 80.11 & 68.48 & 87.75 & 47.42 \\
& \textbf{KR-NFT} & 99.49 & 1.84 & 95.46 & 18.63 & 92.13 & 27.87 & 91.57 & 31.15 & 94.66 & 20.12 \\
 \midrule
{\multirow{5}{*}{ImageNet-V2}} & MCM \cite{ming2022delving} & 91.79 & 45.90 & 89.88 & 50.73 & 86.52 & 56.25 & 81.51 & 69.57 & 87.43 & 55.61 \\  
& NegLabel \cite{jiang2024negative} & 99.40 & 2.47 & 94.46 & 25.69 & 90.00 & 42.03 & 88.46 & 48.90 & 93.08 & 29.77 \\ 
& LoCoOp \cite{miyai2024locoop} & 66.57 & 68.42 & 74.54 & 58.67 & 71.76 & 68.50 & 84.44 & 54.35 & 74.33 & 62.48 \\
& ID-Like \cite{bai2024id} & 93.89 & 33.48 & 82.44 & 67.58 & 85.05 & 61.64 & 91.05 & 35.59 & 88.11 & 49.57\\
& NegPrompt \cite{li2024learning} & 60.73 & 76.19 & 74.46 & 64.52 & 80.16 & 59.41 & 80.88 & 53.55 & 74.06 & 63.42 \\
& SCT \cite{yu2024self} & 94.13 & 25.14 & 93.54 & 28.31 & 89.65 & 37.95 & 85.29 & 54.50 & 90.65 & 36.47 \\
& LAPT \cite{zhang2024lapt} & 99.48 & 1.58 & 93.91 & 27.08 & 90.74 & 41.29 & 89.06 & 45.41& 93.30 & 28.84 \\
& \textbf{KR-NFT} & 99.29 & 3.01 & 94.05 & 30.07 & 90.90 & 38.66 & 90.22 & 44.79 & 93.61 & 29.13 \\
\bottomrule
\end{tabular}
\caption{Unseen styles OOD detection results with ID data of ImageNet-1k and four OOD datasets by using the VITB/16 CLIP encoder.} \label{tab:cross_domain_ood}
% \vspace{-0.2cm}
\end{table*}

% \begin{figure}
% \centering
%     \begin{subfigure}{0.235\textwidth}
%         \includegraphics[width=\linewidth]{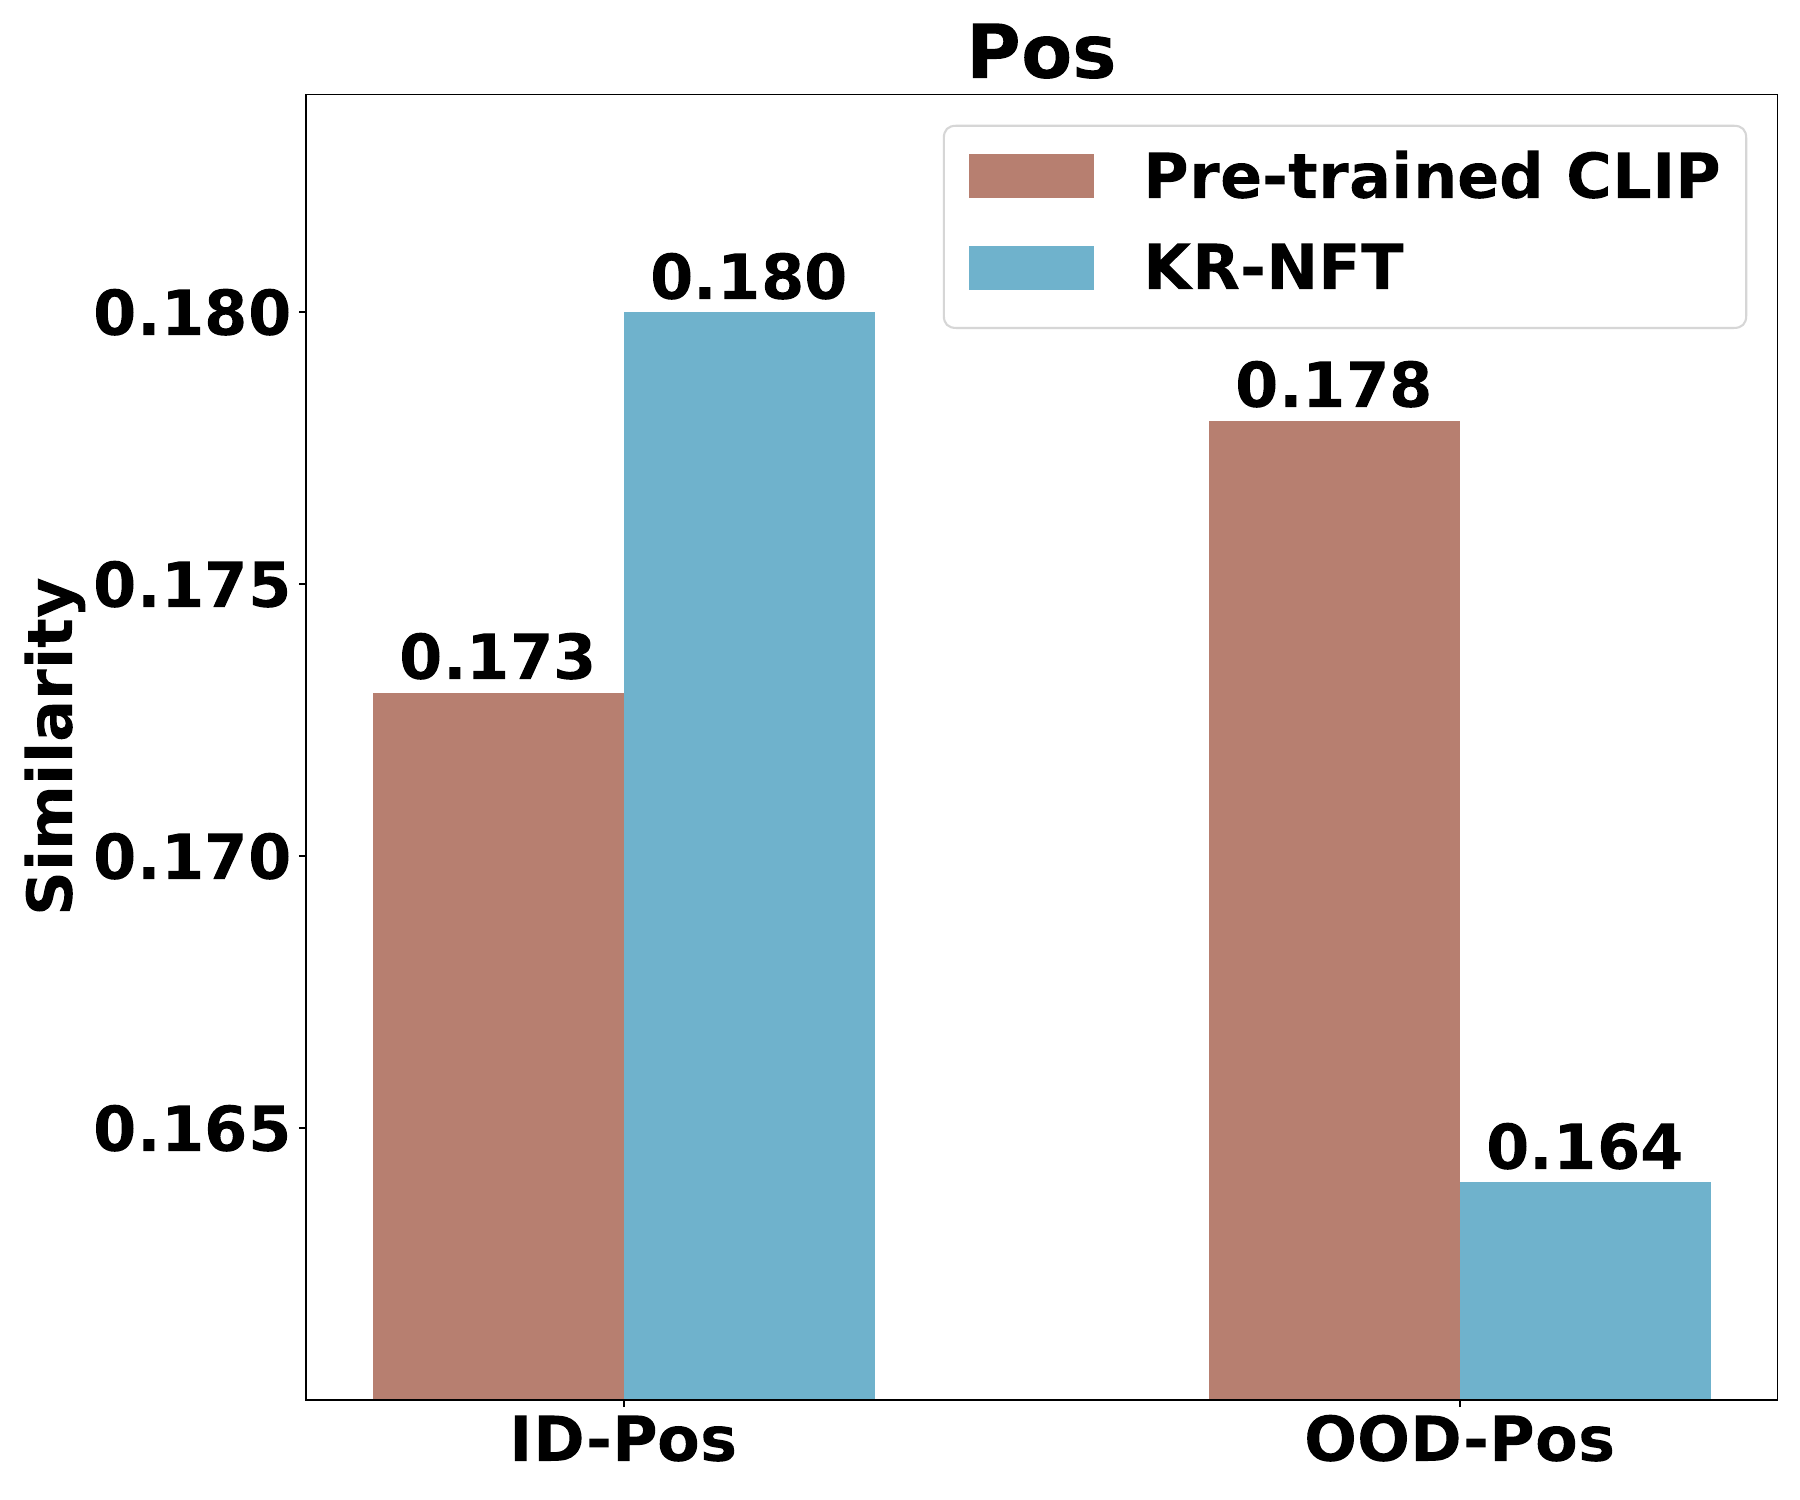}
%         \caption{Similarity to Positive Features}
%         \label{fig:positive_features}
%     \end{subfigure}
%     \begin{subfigure}{0.235\textwidth}
%         \includegraphics[width=\linewidth]{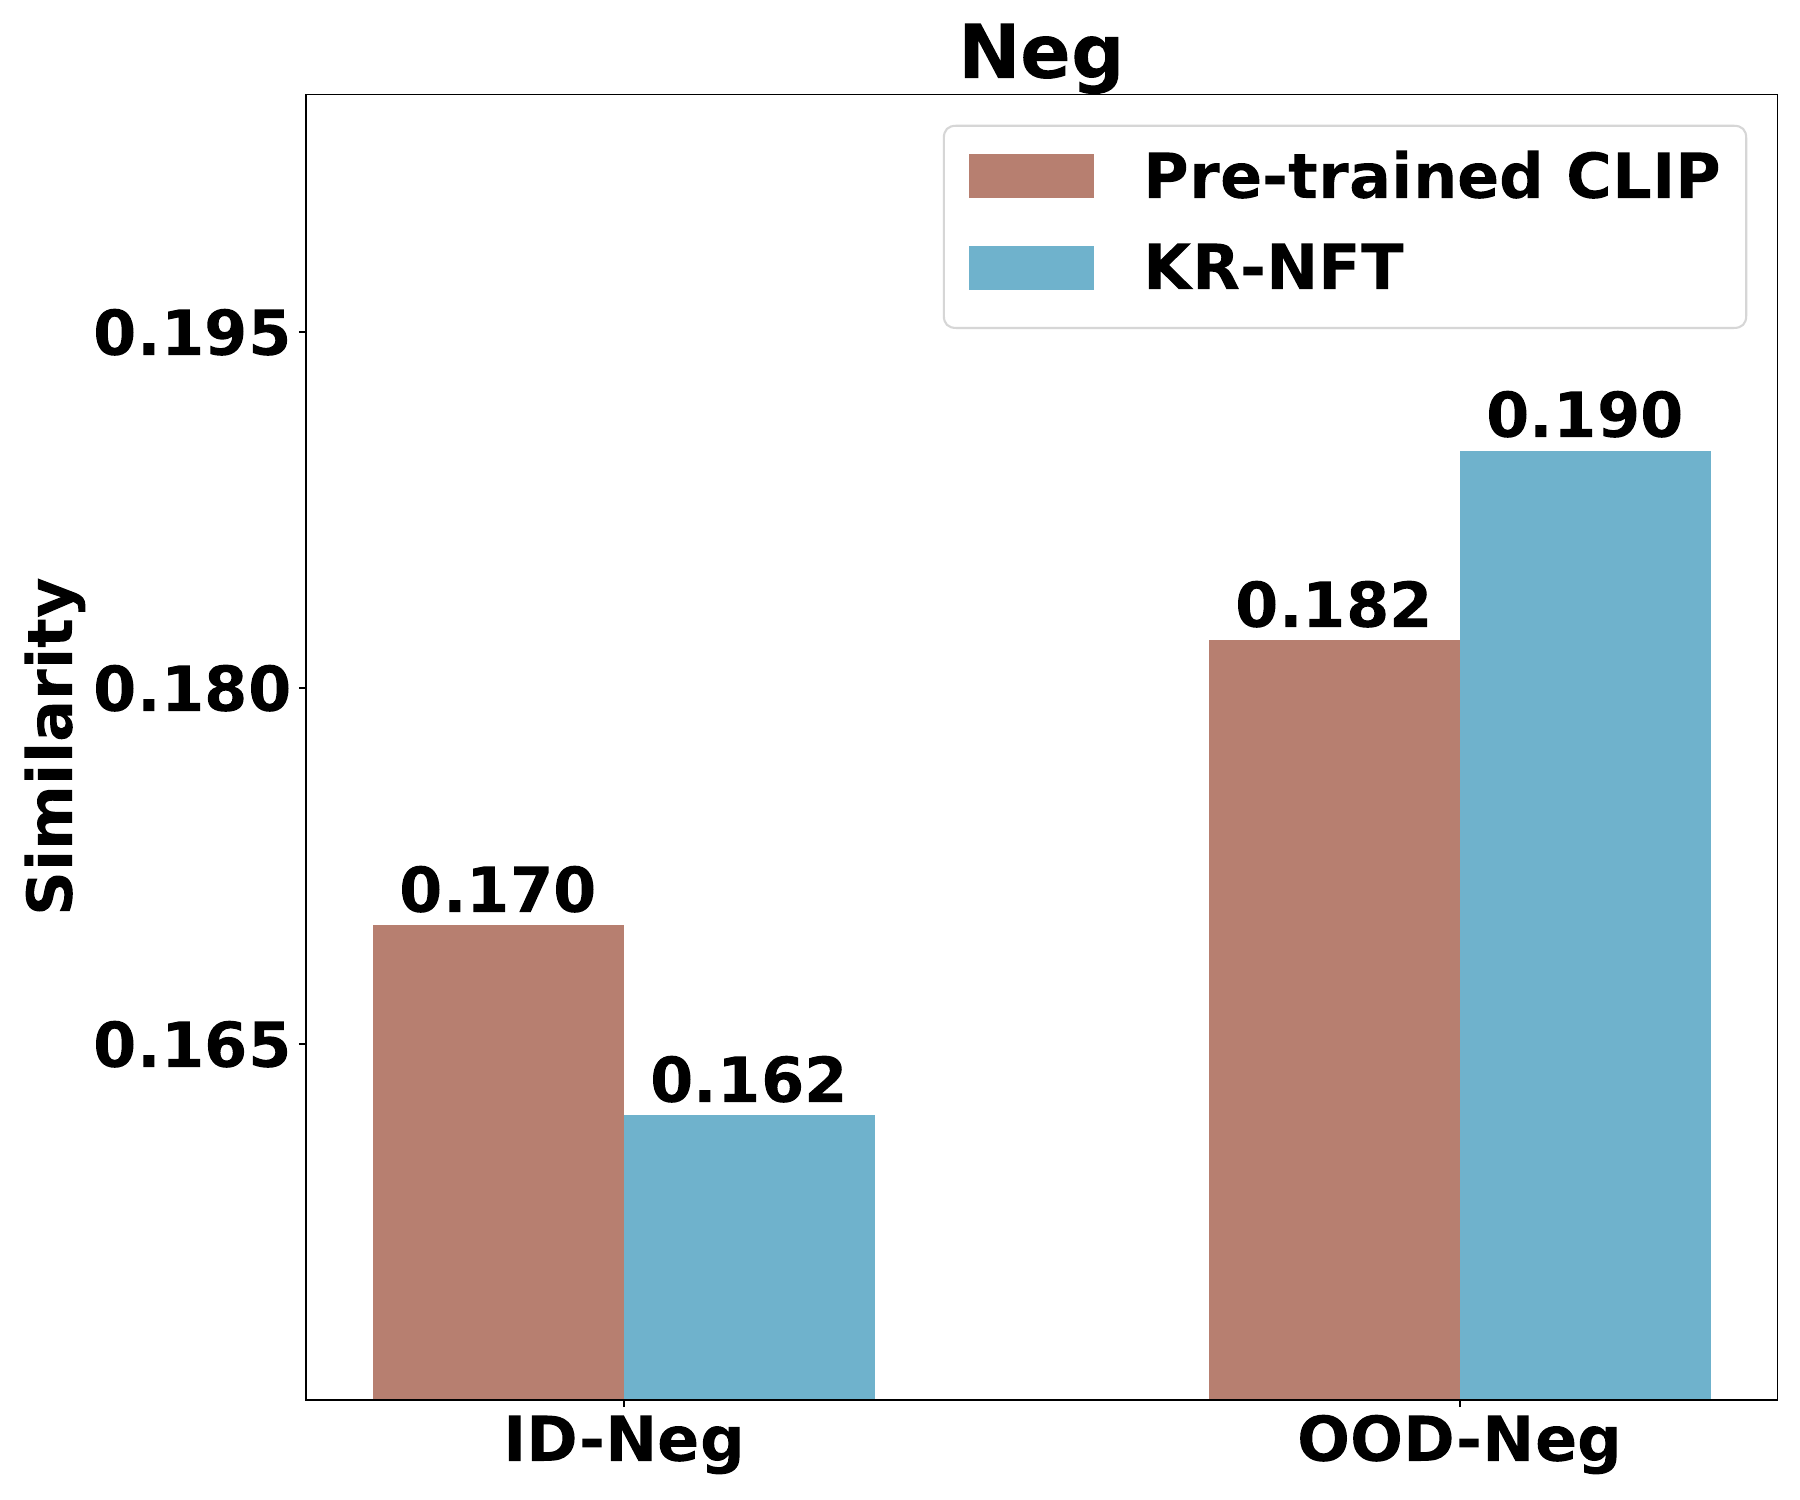}
%         \caption{Similarity to Negative Features}
%         \label{fig:negative_features}
%     \end{subfigure}
%     \vspace{-0.7cm}
%     \caption{
%     Average cosine similarity between ID/OOD image features and positive/negative text features for pre-trained CLIP and our KR-NFT. 
%     Our KR-NFT significantly maximizes the correlation between ID images and positive features, as well as between OOD images and negative features. In this analysis, ImageNet\cite{deng2009imagenet} and SUN\cite{xiao2010sun} are adopted as ID and OOD datasets, respectively.}
%     \vspace{-0.6cm}
%     \label{fig:effectiveness}
% \end{figure}

\clearpage
